# Supplementary material for: Asteria: Deep Learning-based AST-Encoding for Cross-platform Binary Code Similarity Detection
Source: arXiv:2108.06082 source file (2021-08-13)
Supplement: Supplementary file 1 [file appendix.tex]

\begin{appendices}

\onecolumn
\section{} \label{appendix}

\end{appendices}
